# Supplementary material for: Self-Calibrating Gaussian Splatting for Large Field of View Reconstruction
Source: arXiv:2502.09563 source file (2025-04-03)
Supplement: Supplementary file 1 [file supp_crop_fov220.tex]

{
\begin{figure}[t]
    \centering
    \setlength{\tabcolsep}{1pt} % Adjust space between columns if needed
    \begin{tabular}{cc} % 5 columns
        \includegraphics[height=0.2\textwidth]{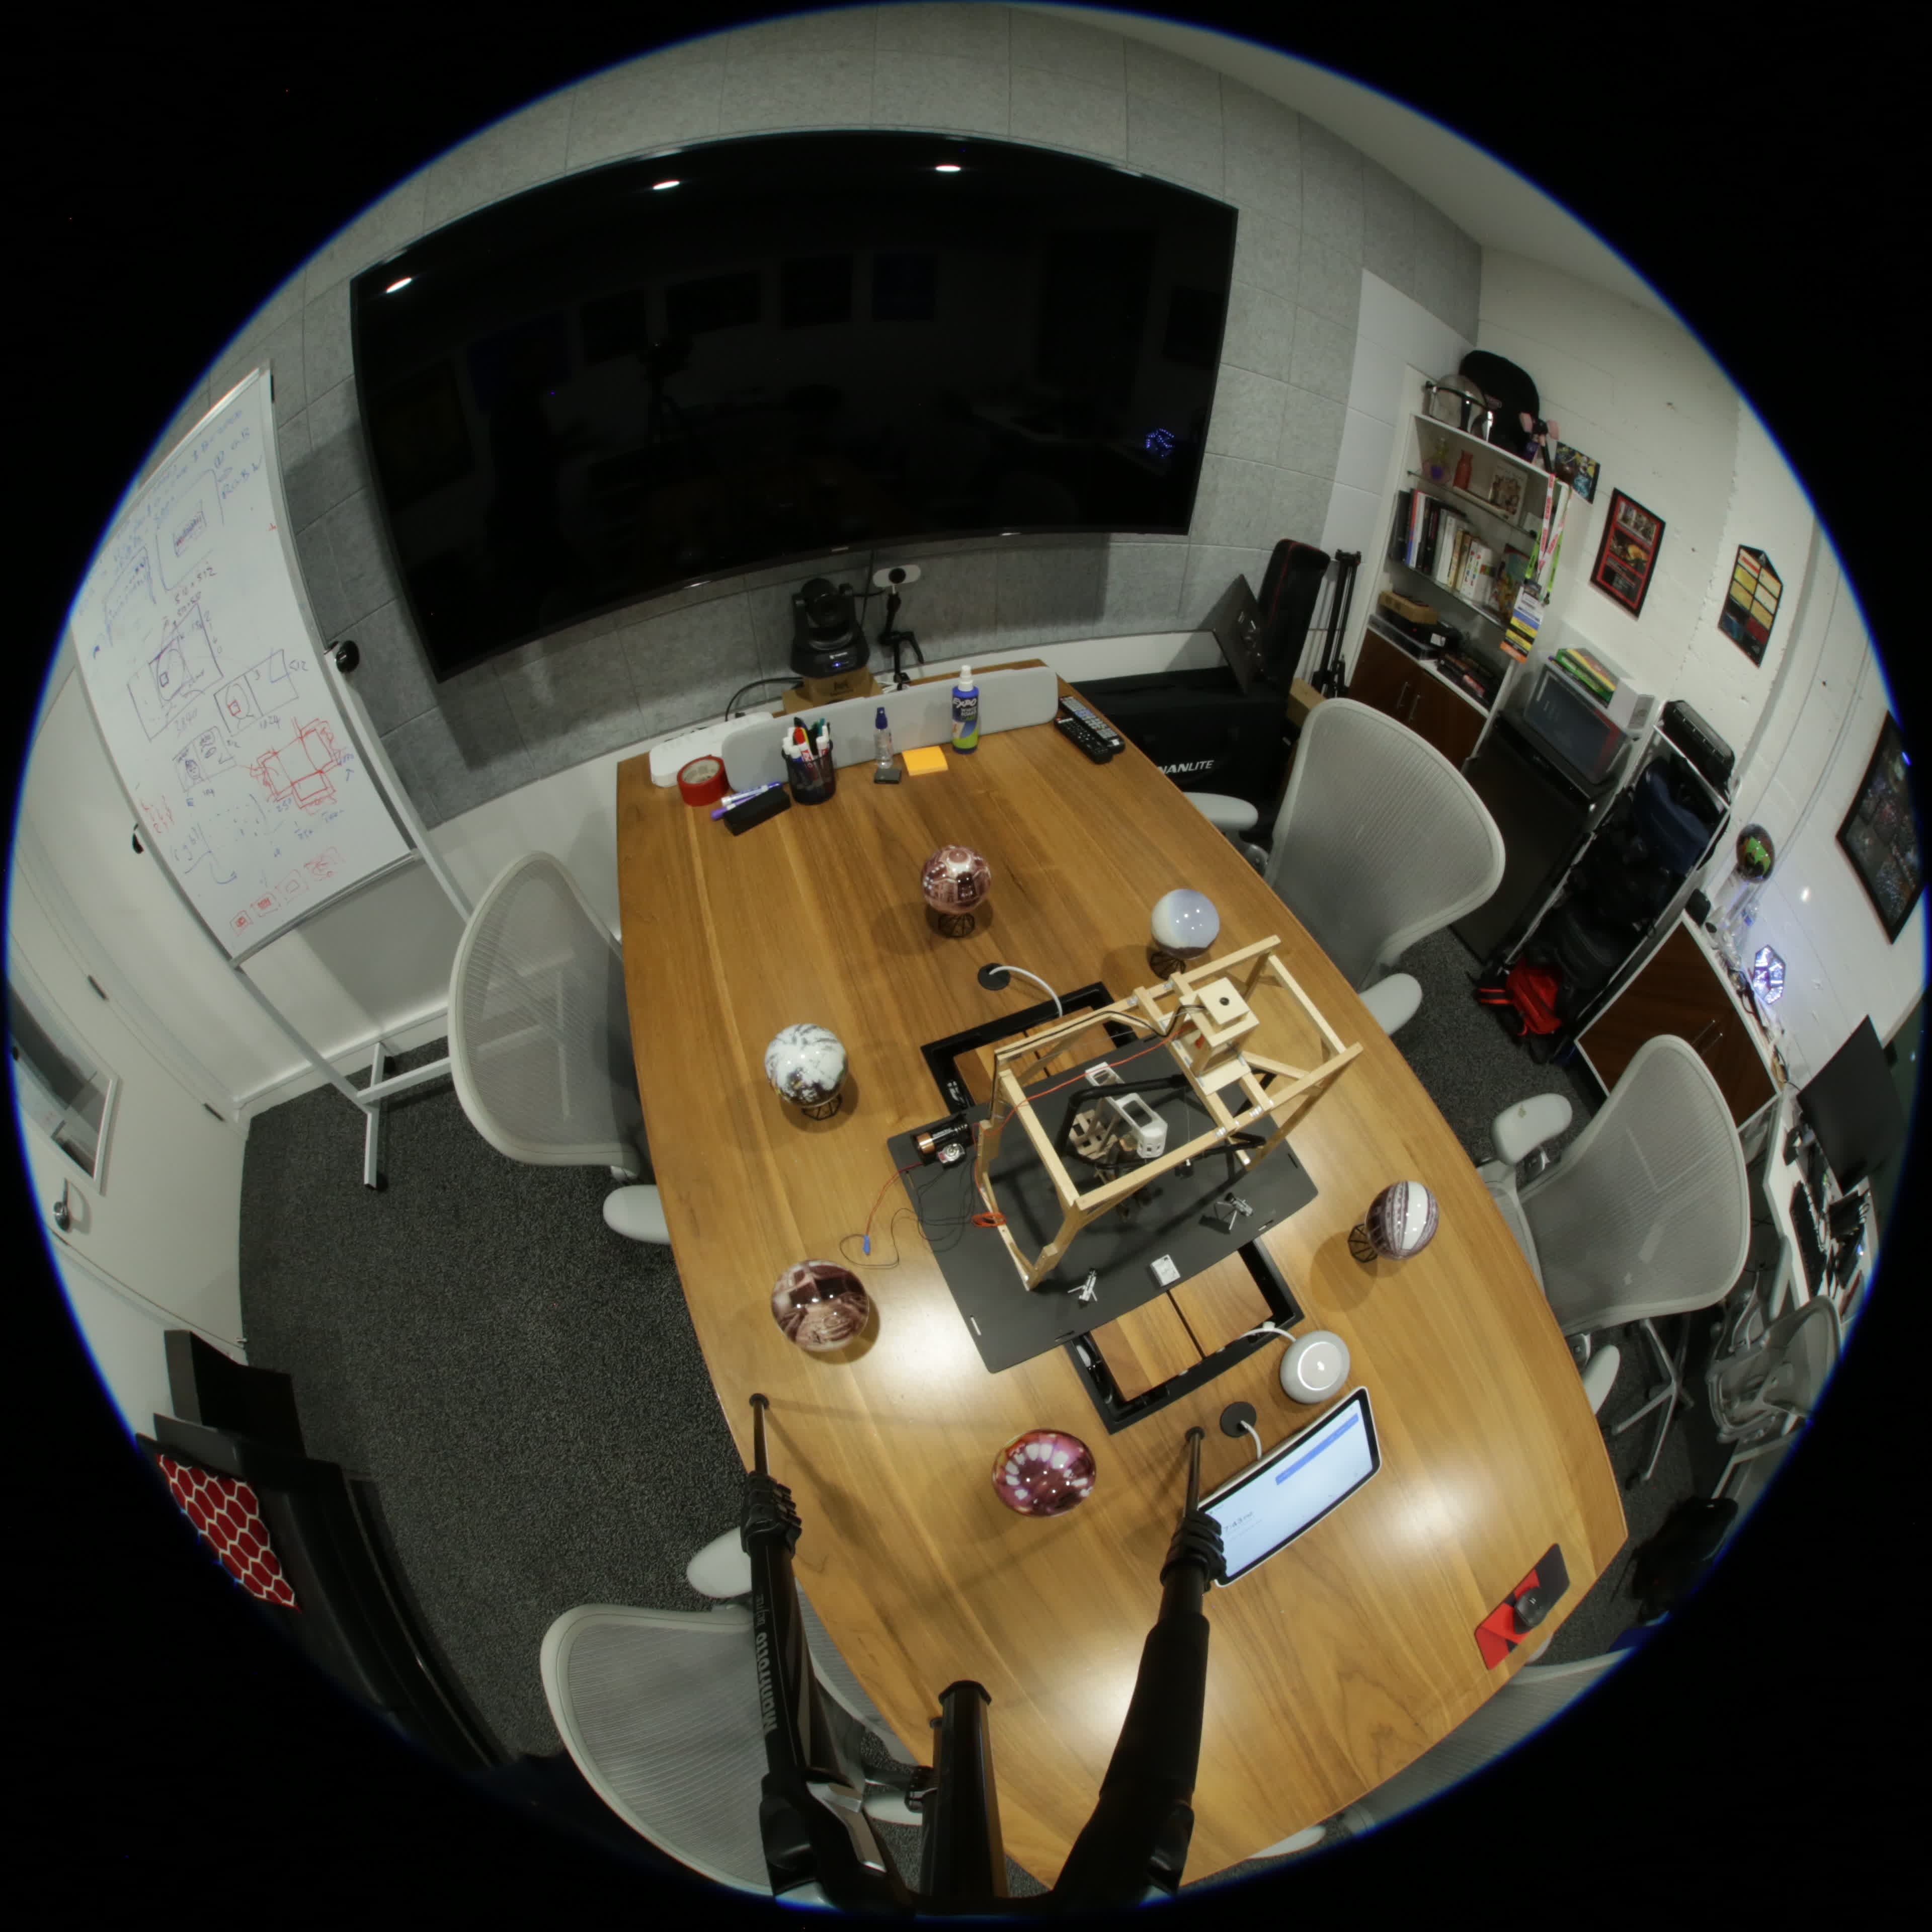} &
         \includegraphics[height=0.2\textwidth]{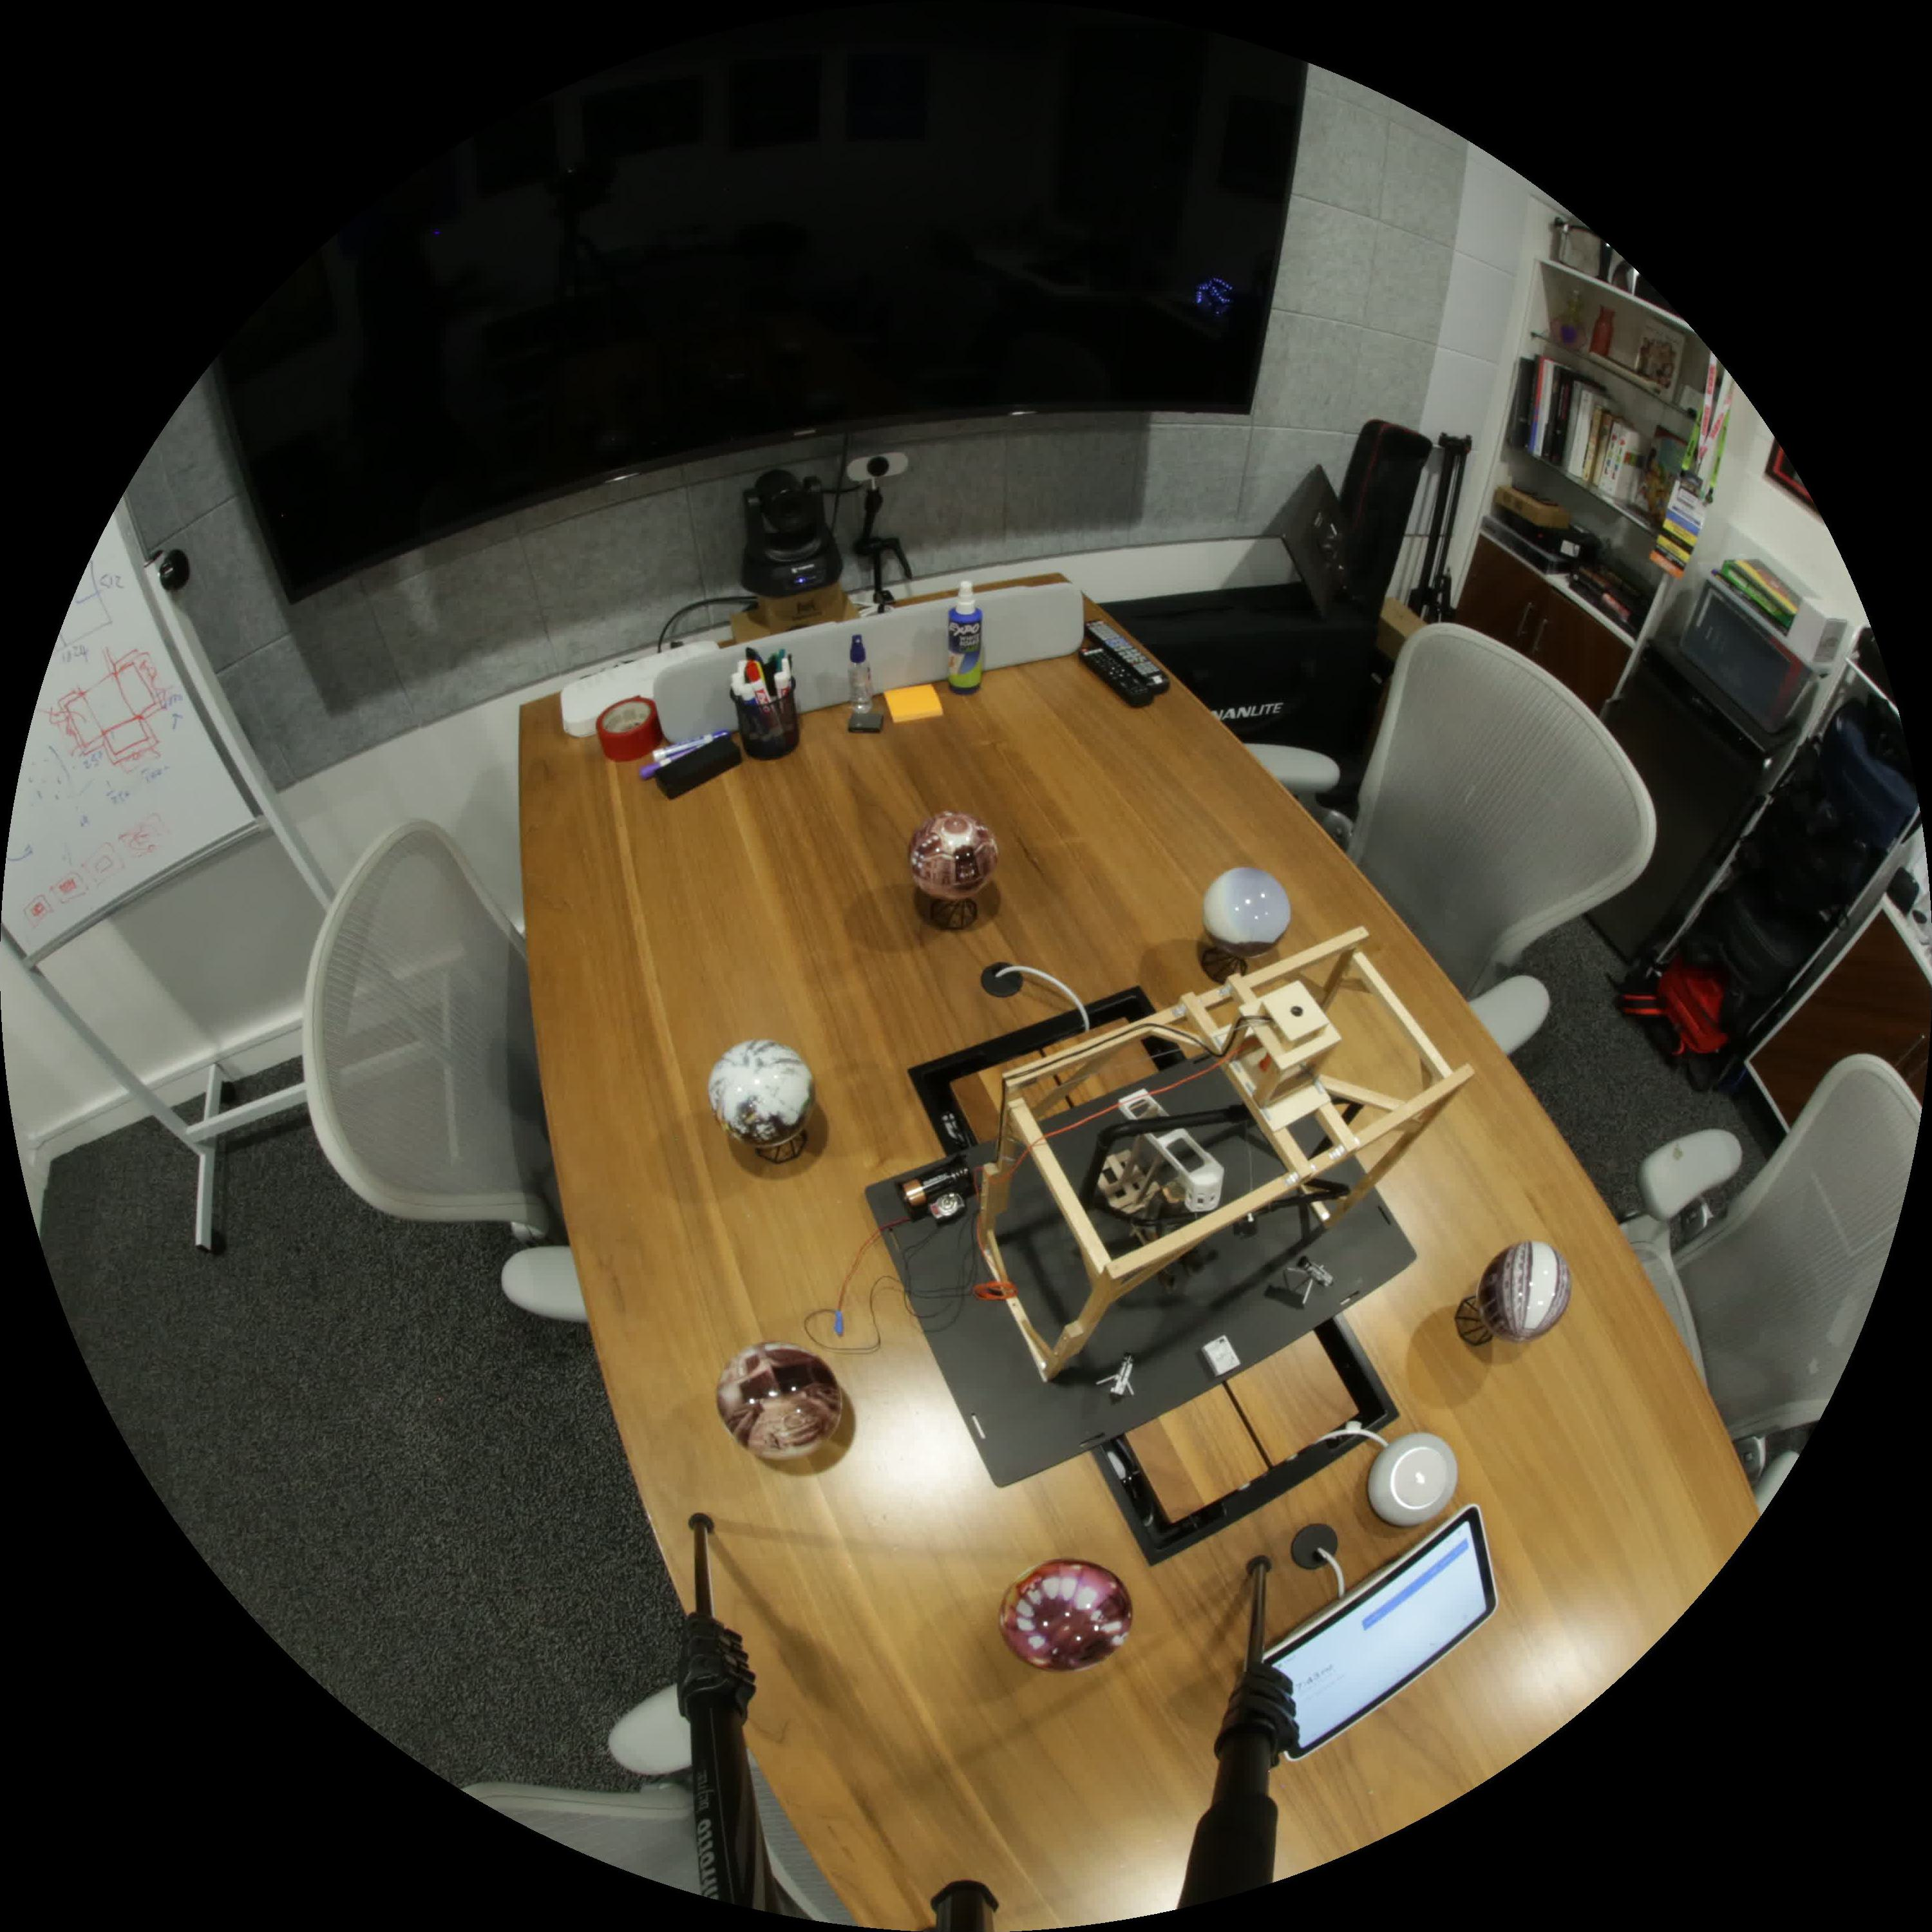} \\

        \multicolumn{1}{c}{(a) Original} & \multicolumn{1}{c}{(b) Cropped}
    \end{tabular}

    \caption{\textbf{Preprocessing of Ultra Wide Angle}. Meike camera we used has a FOV of 220\si{\degree}, which means it project scenes on the back of images plane. In this case, our first step of estimating extrinsic will fail in COLMAP~\cite{schoenberger2016sfm}}

    \label{fig:fov220}

\end{figure}
}
